# Supplementary material for: A Reconnaissance Attack Mechanism for Fixed-Priority Real-Time Systems
Source: arXiv:1705.02561 source file (2017-05-07)
Supplement: Supplementary file 1 [file snp_appendix.tex]

\appendix

\section{Proof of Theorem~\ref{thm:estimate_nk}}
\label{appendix:thm_estimate_nk_proof}
Consider $t_0^i$, $t_1^i$, $t_2^i$, $\cdots$ as the arrival times of task $\tau_i$ and define $\mathcal{S}=\{t_0^i, t_1^i, t_2^i, \cdots\}$. We use the following two lemmas to prove Theorem~\ref{thm:estimate_nk}:
\begin{lemma}
\label{lem:0}
 A busy interval contains the $k^{th}$ task of $\tau_i$ if and only if it contains $t_k^i$ (either as an interior point or as a boundary point).
\end{lemma}
\begin{proof}
The $k^{th}$ task of $\tau_i$ will be released at time $t_k^i$ if there are no tasks with higher priority running at that time, or, will be released immediately after the end of the tasks with higher priority. Hence, in both cases, the system is busy from time $t_k^i$ to at least the finishing time of the $k^{th}$ task of type $i$. Therefore, a busy interval which contains $t_k^i$, contains the $k^{th}$ task of $\tau_i$, and a busy interval that contains the $k^{th}$ task of $\tau_i$, should have started at $t_k^i$ or at a time before $t_k^i$. (Note that the end point of a busy interval cannot belong to $\mathcal{S}$).\\
\end{proof}

\begin{lemma}
\label{lem:1}
If $C(w_k)$ satisfies
\begin{equation}
Np_i<C(w_k)<(N+1)p_i,\hspace{1cm}N=0,1,2,...
\end{equation}
then task $\tau_i$ can only has arrived $N$ or $N+1$ times during the busy interval $w_k$.
\end{lemma}
\begin{proof}
If $Np_i<C(w_k)<(N+1)p_i$, then $w_k$ contains $N$ or $N+1$ points of $\mathcal{S}$. Therefore, by Lemma \ref{lem:0}, task $\tau_i$ can only arrive $N$ or $N+1$ times during the busy interval $w_k$.\\
\end{proof}

\begin{proof}[Proof of Theorem 1]
(i) If $Np_i-c_i\le C(w_k)<Np_i$, then the busy interval cannot contain $N-1$ points from  $\mathcal{S}$, otherwise, a task of type $i$ should have finished in a time interval less that $c_i$ seconds. Therefore, it exactly contains $N$ points from  $\mathcal{S}$.\\
If $Np_i\le C(w_k)<Np_i+c_i$, the start point of the busy interval cannot belong to $\mathcal{S}$ (otherwise, the length of the busy interval should be at least $Np_i+c_i$), therefore, it exactly contains $N$ points from $\mathcal{S}$.\\
Therefore, by Lemma \ref{lem:0}, in both cases, task $\tau_i$ can only has arrived $N$ times during the busy interval.\\
(ii) This part follows from Lemma \ref{lem:1} immediately.
\end{proof}

\subsection{Uniqueness of the Combination}
In this appendix we address the problem of determining under what conditions the task combination found for a busy interval is unique.
The key idea is the following:\\

If we can find two distinct sets of tasks, $I^+$ and $I^-$ such that the sum of the execution times in these two sets are equal, that is,
\begin{equation}
\sum_{i\in I^+}c_i=\sum_{i\in I^-}c_i,
\end{equation}
then, ambiguity (non-unique task combination) is possible, and it will happen for a busy interval $w_k$ of length $C(w_k)$, satisfying,
\begin{equation}
C(w_k)=\sum_{i\in I^+}m_ic_i+\sum_{i\in I^-}(m_i+1)c_i+\sum_{i\notin I^+\cup I^-}n_ic_i
\end{equation}
such that,
\begin{equation}
\label{eq:un}
m_ip_i+c_i\le C(w_k)<(m_i+1)p_i-c_i, \hspace{1cm}\forall i\in I^+\cup I^-
\end{equation}
Note that (\ref{eq:un}) implies that for $i\in I^+\cup I^-$, $N_k(\tau_i)=m_i$ or $m_i+1$.\\
The reason for non-uniqueness of task combination is as follows:
\begin{equation}
\begin{aligned}
&\sum_{i\in I^+}m_ic_i+\sum_{i\in I^-}(m_i+1)c_i+\sum_{i\notin I^+\cup I^-}n_ic_i\\
=&\sum_{i\in I^+}m_ic_i+\sum_{i\in I^-}m_ic_i+\sum_{i\in I^-}c_i+\sum_{i\notin I^+\cup I^-}n_ic_i\\
=&\sum_{i\in I^+}m_ic_i+\sum_{i\in I^-}m_ic_i+\sum_{i\in I^+}c_i+\sum_{i\notin I^+\cup I^-}n_ic_i\\
=&\sum_{i\in I^+}(m_i+1)c_i+\sum_{i\in I^-}m_ic_i+\sum_{i\notin I^+\cup I^-}n_ic_i\\
\end{aligned}
\end{equation}
Therefore, more than one task combinations are possible for the busy interval of length $C(w_k)$.\\

\subsection{Values with Uncertainty}
\label{appendix:values_with_uncertainty}
Let $t_0^i$, $t_1^i$, $t_2^i$, ... be the arrival times of $\tau_i$ and define $\mathcal{S}=\{t_0^i, t_1^i, t_2^i,\cdots\}$. If there is no error in the system we expect $\mathcal{S}$ to be $\{a, a+p_i, a+2p_i,\cdots\}$ for some constant offset $a$. \\
We consider the following scenario:
\begin{itemize}
\item
The $k^{th}$ task of $\tau_i$ arrives at time $a+kp_i+\delta_{i,k}$, where $\{\delta_{i,0}, \delta_{i,1}, \delta_{i,2}, ...\}$ is a sequence of $i.i.d.$ real valued random variables with $|\delta_{i,k}|<\delta_i$, $k=1,2,...$.
\item
The execution time of the $k^{th}$ task of type $i$ is $c_i+\gamma_{i,k}$, where $c_i$ is a deterministic and fixed value and $\{\gamma_{i,0}, \gamma_{i,1}, ...\}$ is a sequence of $i.i.d.$ real valued random variables with $|\gamma_{i,k}|<\gamma_i$, $k=0,1,...$.
\end{itemize}
Figure \ref{fig:unc} shows an example of the arrival of $\tau_i$.\\
\begin{figure}[H]
\centering
\includegraphics[width=1.0\columnwidth]{Figures/rev.pdf}
\caption{}
\label{fig:unc}
\end{figure}

The goal is to find the extension of Theorem 1 for the case that we have uncertainty in the values of task parameters. To this end, we first need the following Lemma:

\begin{lemma}
\label{lem:2}
For $\delta_i\ll p_i$, \\
If $0<C(w_k)<2\delta_i$, then task $\tau_i$ can only has arrived $0$ or $1$ times during the busy interval.\\
Furthermore, if $C(w_k)$ satisfies
\begin{equation}
Np_i+2\delta_i<C(w_k)<(N+1)p_i-2\delta_i,\hspace{1cm}N\ge0
\end{equation}
then task $\tau_i$ can only has arrived $N$ or $N+1$ times during the busy interval $w_k$.
\end{lemma}

\begin{proof}
If $0<C(w_k)<2\delta_i$, then the busy interval contains $0$ or $1$ points of $\mathcal{S}$. Therefore, Lemma \ref{lem:0} in Appendix 1 gives the desired result.\\
If $Np_i+2\delta_i<C(w_k)$, then the busy interval contains more than $N-1$ points of $\mathcal{S}$, and
if $C(w_k)<(N+1)p_i-2\delta_i$, then the busy interval contains less than $N+2$ points of $\mathcal{S}$.
Therefore, by Lemma \ref{lem:0}, task $\tau_i$ can only arrive $N$ or $N+1$ times during the busy interval.\\
\end{proof}

The following theorem is the extension of Theorem 1 for the case that we have uncertainty in the values of execution times and task periods.

\begin{theorem}
\label{thm:uncertainty}
For given values of $C(w_k)$, $p_i$, $c_i$, $\gamma_i$ and $\delta_i$, such that $\gamma_i, \delta_i\ll c_i$,\\
(i) If $C(w_k)$ satisfies
\begin{equation}
(Np_i-c_i+2\delta_i+\gamma_i)^+\le C(w_k)<Np_i+c_i-2\delta_i-\gamma_i,
\end{equation}
then task $i$ can only has arrived $N$ times during the busy interval.\\
(ii) If $C(w_k)$ satisfies
\begin{equation}
Np_i+c_i-2\delta_i-\gamma_i\le C(w_k)<(N+1)p_i-c_i+2\delta_i+\gamma_i,
\end{equation}
then task $i$ can only has arrived $N$ or $N+1$ times during the busy interval.\\
\end{theorem}
\begin{proof}
(i)
If the condition in part (i) holds, the busy interval should exactly contain $N$ points from $\mathcal{S}$; otherwise, either the packet corresponding to the first point or the one corresponding to the last point should have been executed in a time interval less than $c_i-\gamma_i$, which is not possible.\\
Therefore, by Lemma \ref{lem:0}, task $\tau_i$ should have arrived $N$ times during the busy interval.\\
(ii) This part follows from Lemma \ref{lem:2} immediately.\\
\end{proof}

\begin{corollary}
Defining $\hat{c}_i \triangleq c_i-2\delta_i-\gamma_i$, from Theorem \ref{thm:uncertainty},\\\\
(i) If $C(w_k)$ satisfies
\begin{equation}
(Np_i-\hat{c}_i)^+\le C(w_k)<Np_i+\hat{c}_i,
\end{equation}
then task $\tau_i$ can only has arrived $N$ times during the busy interval.\\
(ii) If $C(w_k)$ satisfies
\begin{equation}
Np_i+\hat{c}_i\le C(w_k)<(N+1)p_i-\hat{c}_i,
\end{equation}
then task $\tau_i$ can only has arrived $N$ or $N+1$ times during the busy interval.\\
\end{corollary}

Recall that $N_k(\tau_i)$ is the number of times that task $\tau_i$ has arrived during the busy interval $w_k$.
Therefore, for this busy interval, we have to find $N_k(\tau_i)$'s such that:
\begin{equation}
|\sum_{i}N_k(\tau_i)c_i-C(w_k)|\leq\sum_{i}(\gamma_i\cdot\max{N_k(\tau_i)})
\end{equation}
where by the theorem above, for each value $N_k(\tau_i)$, at most $2$ values are possible, which are distant by $1$.\\

\subsection{Proof of Theorem~\ref{thm:arrival_windows}}
\label{appendix:thm_arrival_windows_proof}

We partition the busy interval as follows:
\begin{equation*}
[a,b]=[a,a+p_i]\cup[a+p_i,a+2p_i]\cup\cdots\cup[a+jp_i,b]
\end{equation*}
In the proof, we will use the fact that by the periodicity assumption, task $\tau_i$ arrives every $p_i$ seconds. Therefore, if we know that there is no arrival at time $t$, then, $t\pm p_i$ also cannot be arrival times.\\
(i) If we know the exact value of $N_k(\tau_i)$, we exactly know in how many of the intervals of the partition above, arrival exists.
There cannot be an arrival in $[a+jp_i-c_i, a+jp_i]$, otherwise, there should be an arrival in the interval $[a-c_i, a]$ and hence, the busy interval cannot start at $a$.
Also, if we know that there is an arrival in the last interval of the partition, we can make the 1-intervals narrower. Note that there cannot be an arrival in $[b-c_i,b]$, otherwise, the busy interval cannot terminate at $b$. Therefore, there should be an arrival in $[a+(N-1)p_i,b-c_i]$.
Therefore, by the periodicity assumption and by shifting $[a+(N-1)p_i,b-c_i]$ by integer multiples of $p_i$ to the left and taking its intersection with other intervals of the partition, we will get the arrival windows.
Therefore, we have (i).\\ 
\noindent
(ii) Using Theorem 1, if $N_k(\tau_i)=N\text{ or }N+1$, then
\begin{equation*}
Np_i+c_i\le C(w_k)\le (N+1)p_i-c_i.
\end{equation*}
Therefore, in the partition, $j=N$. We know there will be arrivals in first $N$ intervals of the partition, but, we cannot say anything about the last interval of the partition. Therefore, we mark the last one as a 0-1-interval, with the consideration that similar to part (i), there cannot be an arrival in $[b-c_i,b]$. This gives us the second expression. 
Also, for other intervals of the partition, 
similar to part (i), there cannot be an arrival in $[a+jp_i-c_i, a+jp_i]$, for $j=1,..,N$. This gives us the first expression.\\

\subsection{Improvement of Theorem~\ref{thm:arrival_windows}}
The following theorem is the improved version of Theorem~\ref{thm:arrival_windows}:
\begin{theorem}
\label{thm:improved}
Considering a task $\tau_i$ and a busy interval $\omega_k$ that has start time $a$ and end time equal to $b$.\\
The partitioning of the busy interval is done by using the following equations:\\

\noindent
(i) If $\tau_i$ has arrived exactly $N$ times during $w_k$:\\

If $\displaystyle N=\Big\lceil \frac{C(w_k)}{p_i} \Big\rceil$, the following segments are \emph{1-interval}:
\begin{equation}
\label{par1}
\overline{A_k(\tau_i)_j} = [a+(j-1)p_i, b-(N-j)p_i-c_i] \hspace{1cm} 1\le j \le N
\end{equation}

Else, the following segments are \emph{1-interval}:
\begin{equation}
\label{par2}
\overline{A_k(\tau_i)_j} = [b-(N+1-j)p_i, a+jp_i-c_i] \hspace{1cm} 1\le j \le N
\end{equation}

\noindent
(ii) If $\tau_i$ may have arrived either $N$ or  $N+1$ times during $w_k$: \\
the following segments are \emph{1-interval}:
\begin{equation}
\label{par3}
\overline{A_k(\tau_i)_j} = [a+(j-1)p_i, a+jp_i-c_i]\hspace{1cm} 1\le j \le N
\end{equation}
and the following segments are \emph{0-1-interval}:
\begin{equation}
\label{par4}
\overline{A_k(\tau_i)_j} = [a+(j-1)p_i, b-c_i]\hspace{1cm}  j=N+1
\end{equation}

\noindent
where $\overline{A_k(\tau_i)_j}$ is the $j^{th}$ arrival window for task $\tau_i$ in busy interval $\omega_k$.\\
In both cases, the remainder of the busy interval is \emph{0-interval}.
\end{theorem}
\begin{proof}
(i) First we note that by Theorem~\ref{thm:estimate_nk}, If $N_k(\tau_i)=N$, then
\begin{equation*}
(N-1)p_i+c_i\le C(w_k)\le(N+1)p_i-c_i.
\end{equation*}
We partition the busy interval as follows:
\begin{equation*}
[a,b]=[a,a+p_i]\cup[a+p_i,a+2p_i]\cup\cdots\cup[a+jp_i,b]
\end{equation*}
If $(N-1)p_i+c_i\le C(w_k)\le Np_i$, or equivalently, $N=\lceil \frac{C(w_k)}{p_i} \rceil$, then $j=N-1$ and there should be an arrival in each interval of the partition above. Also, there cannot be an arrival in $[b-c_i,b]$, otherwise, the busy interval cannot terminate at $b$. Therefore, there should be an arrival in $[a+(N-1)p_i,b-c_i]$.\\
By the periodicity assumption, task $\tau_i$ arrives every $p_i$ seconds, i.e., if we have an arrival at time $t$, then, $t\pm p_i$ is also arrival times. So, shifting $[a+(N-1)p_i,b-c_i]$ by integer multiples of $p_i$ to the left and taking its intersection with other intervals of the partition, we get (\ref{par1}).\\

If $Np_i\le C(w_k)\le (N+1)p_i-c_i$, then $j=N$ and there should not be any arrivals in the last interval of the partition above. Hence, because of the periodicity, the last arrival should be in the interval $[b-p_i, a+Np_i]$. But, If there is an arrival in interval $[a+Np_i-c_i, a+Np_i]$, then there should be an arrival in the interval $[a-c_i, a]$. Therefore, the busy interval cannot start at $a$. This implies that the last arrival should be in the interval $[b-p_i, a+Np_i-c_i]$.\\
Finally, because of the periodicity, by shifting $[b-p_i, a+Np_i-c_i]$ by integer multiples of $p_i$ to the left and taking its intersection with other intervals of the partition, we get (\ref{par2}).\\
\noindent
(ii) Using theorem 1 again, if $N_k(\tau_i)=N\text{ or }N+1$, then
\begin{equation*}
Np_i+c_i\le C(w_k)\le (N+1)p_i-c_i.
\end{equation*}
Therefore, in the partition, $j=N$, and we cannot say anything about the last interval of the partition. So, we mark it as a 0-1-interval, with the consideration that similar to part (i), there cannot be an arrival in $[b-c_i,b]$. This gives as (\ref{par4}). Also, there should be an arrival in all other intervals of the partition, with the consideration that similar to part (i), there cannot be an arrival in $[a+jp_i-c_i, a+jp_i]$, for $j=1,..,N$. This gives as (\ref{par3}).\\
\end{proof}

\subsection{Extra Example for Estimate of $N_k$}
%\vspace{-0.2in}
\begin{example}
\label{ex:Nk_certain}
Consider a busy interval $\omega_k$ with duration $C(\omega_k)=16$ and a task set $\Gamma=\{\tau_1, \tau_2, \tau_3\}$ as follows:
\begin{center}\footnotesize
\begin{tabular}{|c||c|c||c|}
\hline 
 & $p_i$ & $c_i$ & $N_k(\tau_i)$ \\ 
\hline \hline 
$\tau_1$ & 5 & 1 & 3 or 4 \\ \hline 
$\tau_2$ & 17 & 6 & 1 \\ \hline 
$\tau_3$ & 24 & 7 & 0 or 1 \\ \hline 
\multicolumn{4}{r}{$^*C(\omega_k)=16$} \\
%$\tau_0$ & 7 & 2 & 1 or 2 \\ \hline 
%$\tau_1$ & 19 & 6 & 0 or 1 \\ \hline 
%$\tau_2$ & 25 & 11 & 0 \\ \hline 
%\multicolumn{4}{r}{$^*C(\omega_k)=10$} \\
\end{tabular} 
\end{center}
\vspace{-0.10in}

\noindent The above $N_k(\tau_i)$ values are estimated using the conditions of Theorem~\ref{thm:estimate_nk} (Equations (\ref{eqn:Nk_check_1}) and (\ref{eqn:Nk_check_2})). For $\tau_1$, Equation (\ref{eqn:Nk_check_2}) holds when $N_k(\tau_1)=3$ while Equation (\ref{eqn:Nk_check_1}) does not, hence the value of $N_k(\tau_1)$ could be either 3 or 4 implying that $\tau_1$ is likely to have arrived 3 or 4 times during the busy interval $\omega_k$. Likewise, the estimation of $N_k(\tau_3)$ is similar to $N_k(\tau_1)$ except that $\tau_3$ may have arrived 0 or 1 time. For $\tau_2$, Equation (\ref{eqn:Nk_check_1}) holds when $N_k(\tau_2)=1$ and thus we can be sure that it arrived only once during $C(\omega_k)$. We can now use Equation (\ref{eqn:biLength}) to find the combinations of $N_k(\tau_i)$ that can lead to the given busy interval duration $C(\omega_k)$ as shown in the following table:
\vspace{-0.2in}
\begin{center}\footnotesize
\begin{tabular}{|c c c||c|c}
\cline{1-4}
$N_k(\tau_1)$ & $N_k(\tau_2)$ & $N_k(\tau_3)$ & $C(\omega_k)$ &  \\ \cline{1-4} \cline{1-4}
3 & 1 & 0 & 9 &  \\ \cline{1-4} 
3 & 1 & 1 & 16 & $\surd$ matched \\ \cline{1-4} 
4 & 1 & 0 & 10 &  \\ \cline{1-4} 
4 & 1 & 1 & 17 &  \\ \cline{1-4} 
\multicolumn{4}{r}{$^*C(\omega_k)=16$} & \multicolumn{1}{c}{} \\
\end{tabular} 
\end{center}
\vspace{-0.1in}

\noindent In this case, only the combination of $N_k=\{3, 1, 1\}$ satisfies Equation (\ref{eqn:biLength}) for a busy interval length of $C(\omega_k)=16$.
\end{example}

%\newpage

\begin{figure}[t]
    \centering

    \begin{subfigure}[t]{0.49\columnwidth}
        \centering
        \includegraphics[width=1\columnwidth]{Figures/Eva_C3_UtilGroup_ZoomIn/Eva_C3_0001_ZoomIn}
        %\vspace{-\baselineskip}
        \caption{Utilization = [0.0, 0.1]}
        %\vspace{-\baselineskip}
    \end{subfigure}%
        ~ 
    \begin{subfigure}[t]{0.49\columnwidth}
        \centering
        \includegraphics[width=1\columnwidth]{Figures/Eva_C3_UtilGroup_ZoomIn/Eva_C3_0102_ZoomIn}
        %\vspace{-\baselineskip}
        \caption{Utilization = [0.1, 0.2]}
        %\vspace{-\baselineskip}
    \end{subfigure}%
        
    \hfill
            
    \begin{subfigure}[t]{0.49\columnwidth}
        \centering
        \includegraphics[width=1\columnwidth]{Figures/Eva_C3_UtilGroup_ZoomIn/Eva_C3_0203_ZoomIn}
        %\vspace{-\baselineskip}
        \caption{Utilization = [0.2, 0.3]}
        %\vspace{-\baselineskip}
    \end{subfigure}%
        ~ 
    \begin{subfigure}[t]{0.49\columnwidth}
        \centering
        \includegraphics[width=1\columnwidth]{Figures/Eva_C3_UtilGroup_ZoomIn/Eva_C3_0304_ZoomIn}
        %\vspace{-\baselineskip}
        \caption{Utilization = [0.3, 0.4]}
        %\vspace{-\baselineskip}
    \end{subfigure}%
        
    \hfill
            
    \begin{subfigure}[t]{0.49\columnwidth}
        \centering
        \includegraphics[width=1\columnwidth]{Figures/Eva_C3_UtilGroup_ZoomIn/Eva_C3_0405_ZoomIn}
        %\vspace{-\baselineskip}
        \caption{Utilization = [0.4, 0.5]}
        %\vspace{-\baselineskip}
    \end{subfigure}%
        ~ 
    \begin{subfigure}[t]{0.49\columnwidth}
        \centering
        \includegraphics[width=1\columnwidth]{Figures/Eva_C3_UtilGroup_ZoomIn/Eva_C3_0506_ZoomIn}
        %\vspace{-\baselineskip}
        \caption{Utilization = [0.5, 0.6]}
        %\vspace{-\baselineskip}
    \end{subfigure}%
        
    \hfill
        
    \begin{subfigure}[t]{0.49\columnwidth}
        \centering
        \includegraphics[width=1\columnwidth]{Figures/Eva_C3_UtilGroup_ZoomIn/Eva_C3_0607_ZoomIn}
        %\vspace{-\baselineskip}
        \caption{Utilization = [0.6, 0.7]}
        %\vspace{-\baselineskip}
    \end{subfigure}%
        ~ 
    \begin{subfigure}[t]{0.49\columnwidth}
        \centering
        \includegraphics[width=1\columnwidth]{Figures/Eva_C3_UtilGroup_ZoomIn/Eva_C3_0708_ZoomIn}
        %\vspace{-\baselineskip}
        \caption{Utilization = [0.7, 0.8]}
        %\vspace{-\baselineskip}
    \end{subfigure}%
        
    \hfill
        
    \begin{subfigure}[t]{0.49\columnwidth}
        \centering
        \includegraphics[width=1\columnwidth]{Figures/Eva_C3_UtilGroup_ZoomIn/Eva_C3_0809_ZoomIn}
        \vspace{-\baselineskip}
        \caption{Utilization = [0.8, 0.9]}
        %\vspace{-\baselineskip}
    \end{subfigure}%
        ~ 
    \begin{subfigure}[t]{0.49\columnwidth}
        \centering
        \includegraphics[width=1\columnwidth]{Figures/Eva_C3_UtilGroup_ZoomIn/Eva_C3_0910_ZoomIn}
        \vspace{-\baselineskip}
        \caption{Utilization = [0.9, 1.0]}
        %\vspace{-\baselineskip}
    \end{subfigure}
    %\vspace{-\baselineskip}
    \caption{Zoom-in view of precision ratio in each utilization group in \emph{Condition.C}.}
    \label{fig:eva_c3_util_group_10groups}
    \vspace{-\baselineskip}
\end{figure}

\subsection{Compact Scheduling Translator}\label{subsec::CST}
In order to reconstruct the schedule for a specified busy interval, a \emph{compact scheduling translator} is used to convert arrival times of participating tasks to corresponding start times - the instant when a task actually starts running.

Similar to a regular fixed-priority scheduler, it applies the scheduling algorithm to organize the sequence and preemption of each job execution. However, in contrast to a real scheduler, it omits the real execution and does only the estimation of the start times. The translator starts with the first arrival in the busy interval and stops when there is nothing is to be scheduled in the simulation queue, which is equivalent to the close of the given busy interval. The detailed algorithm is presented in Algorithm~\ref{algo:scheduleTranslator}.

\begin{algorithm}
\caption{Compact Scheduling Translator}
\label{algo:scheduleTranslator}
\begin{algorithmic}[1]
\STATE \{\textit{$A_k$: arrival time array of $\omega_k$}\}
\STATE \{\textit{$S_k$: task start time array of $\omega_k$}\}
\STATE \{\textit{$AQueue$: arrival queue storing initial arrival times}\}
\STATE \{\textit{$SQueue$: ready queue for suspended jobs}\}
\STATE \{\textit{$A_{this}$: arrival time of current running job $\tau_{this}$}\}
\STATE \{\textit{$A_{next}$: arrival time of next job $\tau_{next}$}\}
\STATE \{\textit{$c_{this}$: remaining execution time of job $\tau_{this}$}\}
\STATE \{\textit{E{\&}HP: "earliest and highest priority job"}\}
\STATE {}
\STATE \textit{$AQueue.pushAll(A_k)$}
\STATE \textit{$A_{this} \leftarrow$ AQueue.pop(E{\&}HP)}
\STATE \textit{$S_k.add(\{A_{this}, \tau_{this}\})$}
\WHILE {\textit{$AQueue$ and $SQueue$ are not empty}}
	\STATE \textit{$A_{next} \leftarrow$ \{AQueue, SQueue\}.pop(E{\&}HP) }
	\IF {\textit{$(A_{this}+c_{this}) > A_{next}$}}
		\STATE \textit{$c_{this} \leftarrow c_{this}-(A_{next}-A_{this})$}
		\STATE \textit{SQueue.push($\tau_{this}, A_{next}, c_{this}$)}
	\ENDIF
	
	\IF {\textit{$A_{next}$ is from AQueue}}
		\STATE \textit{$S_k.add(\{A_{next}, \tau_{next}\})$}
	\ENDIF
	\STATE \textit{$A_{this} \leftarrow A_{next}$}
\ENDWHILE
\RETURN {$S_k$}
\end{algorithmic}
\end{algorithm}
