# Supplementary material for: A Reconnaissance Attack Mechanism for Fixed-Priority Real-Time Systems
Source: arXiv:1705.02561 source file (2017-05-07)
Supplement: Supplementary file 2 [file appendix.tex]

%\newpage
\appendix

\section{Appendix: Task with Variation}
\label{appendix:values_with_uncertainty}
Let $t_0^i$, $t_1^i$, $t_2^i$, ... be the arrival times of $\tau_i$ and define $\mathcal{S}=\{t_0^i, t_1^i, t_2^i,\cdots\}$. If there is no error in the system we expect $\mathcal{S}$ to be $\{a, a+p_i, a+2p_i,\cdots\}$ for some constant offset $a$. \\
We consider the following scenario:
\begin{itemize}
\item
The $h^{th}$ task of $\tau_i$ arrives at time $a+hp_i+\theta_{i,h}$, where $\{\theta_{i,0}, \theta_{i,1}, \theta_{i,2}, ...\}$ is a sequence of $i.i.d.$ real valued random variables with $|\theta_{i,h}|<\theta_i$, $h=1,2,...$.
\item
The execution time of the $h^{th}$ task of type $i$ is $c_i+\gamma_{i,h}$, where $c_i$ is a deterministic and fixed value and $\{\gamma_{i,0}, \gamma_{i,1}, ...\}$ is a sequence of $i.i.d.$ real valued random variables with $|\gamma_{i,h}|<\gamma_i$, $h=0,1,...$.
\end{itemize}

\begin{comment}
Figure \ref{fig:unc} shows an example of the arrival of $\tau_i$.\\
\begin{figure}[H]
\centering
\includegraphics[width=1.0\columnwidth]{Figures/rev.pdf}
\caption{}
\label{fig:unc}
\end{figure}
\end{comment}

The goal is to find the extension of Theorem 1 for the case that we have uncertainty in the values of task parameters. To this end, we first need the following Lemma:

\begin{lemma}
\label{lem:2}
For $\theta_i\ll p_i$,
if $0<l_k<2\theta_i$, then task $\tau_i$ can only has arrived $0$ or $1$ times during the busy interval.
Furthermore, if $l_k$ satisfies
%\begin{equation}
%$Np_i+2\theta_i<l_k<(N+1)p_i-2\theta_i,\hspace{1cm}N\ge0$,
$Np_i+2\theta_i<l_k<(N+1)p_i-2\theta_i,N\ge0$,
%\end{equation}
then task $\tau_i$ can only has arrived $N$ or $N+1$ times during the busy interval $w_k$.
\end{lemma}

\begin{proof}
If $0<l_k<2\theta_i$, then the busy interval contains $0$ or $1$ points of $\mathcal{S}$. Therefore, Lemma \ref{lem:0} gives the desired result.\\
If $Np_i+2\theta_i<l_k$, then the busy interval contains more than $N-1$ points of $\mathcal{S}$, and
if $l_k<(N+1)p_i-2\theta_i$, then the busy interval contains less than $N+2$ points of $\mathcal{S}$.
Therefore, by Lemma \ref{lem:0}, task $\tau_i$ can only arrive $N$ or $N+1$ times during the busy interval.\\
\end{proof}

\vspace{-0.5\baselineskip}
The following theorem is the extension of Theorem 1 for the case that we have uncertainty in the values of execution times and task periods.

\begin{theorem}
\label{thm:uncertainty}
For given values of $l_k$, $p_i$, $c_i$, $\gamma_i$ and $\theta_i$, such that $\gamma_i, \theta_i\ll c_i$,\\
(i) If $l_k$ satisfies
%\begin{equation}
$(Np_i-c_i+2\theta_i+\gamma_i)^+\le l_k<Np_i+c_i-2\theta_i-\gamma_i$,
%\end{equation}
then task $i$ can only has arrived $N$ times during the busy interval.\\
(ii) If $l_k$ satisfies
%\begin{equation}
$Np_i+c_i-2\theta_i-\gamma_i\le l_k<(N+1)p_i-c_i+2\theta_i+\gamma_i$,
%\end{equation}
then task $i$ can only has arrived $N$ or $N+1$ times during the busy interval.\\
\end{theorem}
\vspace{-1\baselineskip}
\begin{proof}
(i)
If the condition in part (i) holds, the busy interval should exactly contain $N$ points from $\mathcal{S}$; otherwise, either the packet corresponding to the first point or the one corresponding to the last point should have been executed in a time interval less than $c_i-\gamma_i$, which is not possible.
Therefore, by Lemma \ref{lem:0}, task $\tau_i$ should have arrived $N$ times during the busy interval.\\
(ii) This part follows from Lemma \ref{lem:2} immediately.\\
\end{proof}
